# Supplementary material for: RPP: Automatic Proof of Relational Properties by Self-Composition
Source: arXiv:1606.00678 source file (2017-02-06)
Supplement: Supplementary file 1 [file appendix.tex]

\subsection{Introduction}

This tool demo presents a new \framac plugin \toolname that allows to prove relational 
properties by using the technique of self-composition.
The \toolname tool is available for the reviewers in a Linux virtual machine at
\url{http://pathcrawler-online.com/RPP-VM-TACAS2017.ova}.
In case of any access issue, the authors can 
also provide the virtual machine on request by the PC Chairs.

\framac is a platform dedicated to the analysis of source code written in C. The 
\framac platform gathers several analysis techniques into a single collaborative 
extensible framework. \toolname will work like a preprocessor for the deductive 
verification tool \Wp.
The first part of the demo will thus give a brief overview of \framac itself,
including the \Wp plugin, and of the ACSL specification language used normally
by the tool. We will then present a simple instance of a relational property and
explain why ACSL and \Wp are not sufficient to prove it. Then we will show how
\toolname's proposed solution can successfully handle this issue.

\subsection{Proof and use of relational properties}

\paragraph{Example 1}
In this example we present an application of \toolname on a simple relational property: 
the monotonicity of a function \lstinline{f}, similar to what is presented in
Figure~\ref{fig:ex1}a:

\begin{figure}[htbp]
\centering
\includegraphics[scale=0.35]{"Capture new project".png}
\caption{Screenshot of \framac 's GUI after the execution of the \toolname plugin. 
}
\label{fig:GUI2}
\end{figure}

\begin{center}
\lstset{basicstyle=\scriptsize\ttfamily,}
\begin{scriptsize}
$\forall \ int \ x1,x2; x1 < x2 \Rightarrow$ \lstinline{\call(f1,x1)} $<$ \lstinline{\call(f1,x2)}
\end{scriptsize}
\lstset{basicstyle=\normalsize\ttfamily,}
\end{center}

Runing \toolname on the source of \lstinline{f} will output the result presented 
Figure \ref{fig:GUI2}. The new project contains the function \lstinline{f} with the generated 
\lstinline{ensures} clause, the generated axiomatic definition and the generated wrapper 
function (\lstinline{relational_wrapper_- function}). The \lstinline{assert} and \lstinline{assigns} clauses are not yet proved, while 
the lemma is ``valid under condition'' (depending on the validity of the assertion).

It is now possible to prove the relational property by proving the validity of the 
\lstinline{assert} clause in function \lstinline{relational_wrapper_1}
using \Wp. If the \lstinline{assert} 
clause is proven valid, the lemma status switches automatically to valid
as shown by Figure \ref{fig:GUI4}.

\begin{figure}[htbp]
\centering
\includegraphics[scale=0.35]{"Capture over properties proven".png}
\caption{Screenshot of \framac GUI after the proof of the \lstinline{assert}
and the \lstinline{assigns} clauses  with \Wp.
The status of the lemma is valid since the status icon turns from half green, 
half orange, to fully green.}
\label{fig:GUI4}
\end{figure}

\vspace{-0.1cm}
\smallskip\noindent
\paragraph{Example 2}
Next, the demo will show the ability to use relational
properties for proving other properties.
We consider the cryptographic functions presented Figure \ref{fig:ex6}, and function 
\lstinline{f} presented Figure \ref{fig:GUI9} using this cryptographic function. For reason of 
simplicity and readability, we consider the cryptographic functions coming 
from a library. In other words, we only have their prototype, not their
implementation and the relational properties are in fact their specification.
This example will therefore also show the capacity of RPP to treat software relying on 
library or hardware-provided functions with specified relational properties.

%% %============================
%% \begin{figure}[!h]
%%   \lstset{basicstyle=\scriptsize\ttfamily,mathescape=true}
%%   \lstinputlisting[firstline=1, lastline=8]{Chiffre_de_Cesar.c}
%%     \vspace{-1mm}
%%   \vspace{-3mm}
%% \caption{The encrypting function \lstinline{Encrypt} and the defintion of 
%% struct \lstinline{sentence}}\label{fig:ex5}
%% \end{figure}
%% %============================

%============================
\begin{figure}[!h]
  \lstset{basicstyle=\scriptsize\ttfamily,mathescape=true}
  \lstinputlisting[firstline=1, lastline=23]{Chiffre_de_Cesar.c}
    \vspace{-1mm}
  \vspace{-3mm}
\caption{The encrypting function \lstinline{Encrypt} and the decrypting 
function \lstinline{Decrypt} with the relational property. The defintion of 
struct \lstinline{sentence} and the predicate \lstinline{is_eq}.
And the declaration of function \lstinline{do_something_wih_message.}}\label{fig:ex6}
\end{figure}
%============================

The relational property on top of function prototype \lstinline{Decrypt}, specifies that any
message, encrypted with function \lstinline{Encrypt} and then 
decrypted by \lstinline{Decrypt}, will be
equal to its initial value, provided the same key is used in both operations:

\begin{center}
\lstset{basicstyle=\scriptsize\ttfamily,}
\begin{scriptsize}
$\forall \ Msg,Key;Decrypt(Encrypt(Msg,Key),Key)=Msg$
\end{scriptsize}
\lstset{basicstyle=\normalsize\ttfamily,}
\end{center}
\vspace{-0.07cm}
The postcondition of \lstinline{f} specifies that the result of the function call must be equal to 
the message given as parameter. The body of \lstinline{f} is very simple, but the cryptographic 
functions may have a more complex body and so a more complexe behavior specification. But, thanks to 
the relational properties and \toolname, the interesting function behavior  of \lstinline{Encrypt} 
and \lstinline{Decrypt} is translated, and allows the proof of the postcondition 
(Figure \ref{fig:GUI9}).

\begin{figure}[!hbp]
\centering
\includegraphics[scale=0.35]{"Cryp result".png}
\caption{Screenshot of \framac GUI after the proof of the \lstinline{ensures} clause with \Wp}
\label{fig:GUI9}
\end{figure}

\subsection{Extensions of self-composition}
\paragraph{Example 3} Finally, we show how \toolname goes beyond
self-composition technique. For that, we consider the well known
linear algebra property that is the transpose of the sum of two matrices is the
sum of the transpose of the matrices:

\begin{center}
\lstset{basicstyle=\scriptsize\ttfamily,}
\begin{scriptsize}
$(A + B)^T = (A^T + B^T)$.
\end{scriptsize}
\lstset{basicstyle=\normalsize\ttfamily,}
\end{center}

Figure \ref{fig:exa11} and \ref{fig:exa12} present the transpose function \lstinline{trans} and 
the sum function \lstinline{sum} with the relational specification. The equality between the two
matrices is defined by using predicate \lstinline{is_eq_line} (not given here) defining equality 
between columns \lstinline{i} of the two matrixes. Proving this property is like proving any other relational 
property: calling \toolname and checking the validity of the \lstinline{assert} clause and some 
loop invariant.

%============================
\begin{figure}[!h]
  \lstset{basicstyle=\scriptsize\ttfamily,mathescape=true}
  \lstinputlisting[firstline=15, lastline=32]{matrix3.c}
    \vspace{-1mm}
  \vspace{-3mm}
\caption{The transpose function \lstinline{trans}}  \label{fig:exa11}
\end{figure}
%============================

Indeed, \toolname can manage relational properties invoking any finite number of function calls
of possibly dissimilar functions with possible nested calls.
In the case of our linear algebra property, we have five function calls: two calls with three nested calls.

%============================
\begin{figure}[!h]
  \lstset{basicstyle=\scriptsize\ttfamily,mathescape=true}
  \lstinputlisting[firstline=34, lastline=52]{matrix3.c}
    \vspace{-1mm}
  \vspace{-3mm}
\caption{The \lstinline{sum} function and the relational property}\label{fig:exa12}
\end{figure}
%============================

Figure \ref{fig:GUI10} show the inlining of \lstinline{sum} in the case of $A^T + B^T$. 
\lstinline{local_variable_- relational_2} and \lstinline{local_variable_relational_3} represent 
respectively the result of $A^T$ and $B^T$. Loop invariants are automatically inlined by
RPP into the wrapper function to make possible the automatic proof of the \lstinline{assert} 
clause. The \lstinline{assert} clause is generated with logic variable 
\lstinline{return_variable_relationa- l_1} and \lstinline{return_variable_relational_2} corresponding 
to the result of the two traces, respectively $(A + B)^T$ and $A^T + B^T$.

\begin{figure}[!h]
\centering
\includegraphics[scale=0.35]{"Capture transformation".png}
\caption{Screenshot of \framac GUI after the call to \toolname: Zoom on the end of the 
generated \lstinline{wrapper} function}
\label{fig:GUI10}
\end{figure}

%% \smallskip\noindent
%% \textbf{Exemple 2} provide the proof of a relational property with three call traces, two nested 
%% calls and some arithmetic operation in the call parameter. This example show the possibilities of 
%% the extend ACSL grammar to write complexe properties.

%% %============================
%% \begin{figure}[!hbp]
%%   \lstset{basicstyle=\scriptsize\ttfamily,mathescape=true}
%%   \lstinputlisting[firstline=1, lastline=17]{multi_trace.c}
%%     \vspace{-1mm}
%%   \vspace{-3mm}
%% \caption{Verification of equals result between function \lstinline{g},
%%  \lstinline{f} and \lstinline{h}}\label{fig:exa13}
%% \end{figure}
%% %============================

\subsection{Conclusion}
Thus, through the different examples chosen for the demo, we hope to convince the public of the interest of our tool RPP to prove relational properties.
In short, RPP takes advantage on the maturity of the Frama-C platform by transforming relational properties into  properties likely to be proven with WP plugin.
We will complete the  demo with some properties that cannot yet be processed by RPP and that will be the subject of future work.

% Local Variables:
% compile-command: "pdflatex main.tex"
% mode: latex
% TeX-master: t
% TeX-PDF-mode: t
% mode: flyspell
% ispell-local-dictionary: "american"
% End:
